# Supplementary material for: Predicting complete basis set limit quasiparticle energies from triple-$\zeta$ calculations
Source: arXiv:2511.22462 ancillary file (2025-11-27)
Supplement: Supplementary file 1 [file SI.pdf]

# Supporting Information to Predicting complete basis set limit quasiparticle energies from triple-$\zeta$ calculations

Dario Baum, Lucas Visscher, and Arno Förster*

*Theoretical Chemistry, Vrije Universiteit Amsterdam, De Boelelaan 1105, 1081 HV Amsterdam, The Netherlands*

E-mail: a.t.l.foerster@vu.nl

## Extrapolation Parameters

In the following we list the fitted extrapolation parameters for the GTO and STO basis sets. Tab. S1, S2 and S3 list the numbers of fit and test samples, extrapolation parameters as well as the MAEs between the predicted CBS limit energies based on cc-pVDZ, cc-pVTZ and cc-pVQZ calculations and the reference energies on the test sets. Tab. S4, S5 and S6 show the numbers of fit and test samples, extrapolation parameters as well as the MAEs between the predicted 5Z GTO energies based on different STO basis sets and the reference cc-pV5Z energies (instead of CBS energies as discussed in the main text). Note that for qs*GW* with STO basis sets, the QP energies from the first qs*GW* iteration are extrapolated to the corresponding GTO 5Z reference. In all other cases, the converged QP energies are used for the extrapolation.

Table S1: Numbers of fit and test samples, fitted extrapolation parameters and MAEs on the test sets for $G_0W_0$ and different GTO basis sets.

| Basis Set | Molecules | $n_{\text{train}}$ | $n_{\text{test}}$ | $\alpha_0$ | $\alpha_1$ | MAE [eV] |
|---|---|---|---|---|---|---|
| cc-pVDZ | General | 108 | 27 | 0.5885 | −0.3731 | 0.0315 |
| | Organic | 112 | 28 | 0.3804 | −0.3397 | 0.0384 |
| cc-pVTZ | General | 128 | 32 | 0.5647 | −0.2641 | 0.0236 |
| | Organic | 253 | 64 | 0.5493 | −0.2601 | 0.0331 |
| cc-pVQZ | General | 128 | 32 | 0.3559 | −0.1616 | 0.0254 |
| | Organic | 253 | 64 | 0.3753 | −0.1607 | 0.0283 |

Table S2: Numbers of fit and test samples, fitted extrapolation parameters and MAEs on the test sets for $\Sigma^{BSE}@L^{BSE}$ and different GTO basis sets.

| Basis Set | Molecules | $n_{\text{train}}$ | $n_{\text{test}}$ | $\alpha_0$ | $\alpha_1$ | MAE [eV] |
|---|---|---|---|---|---|---|
| cc-pVDZ | General | 115 | 29 | 0.4182 | −0.2743 | 0.0358 |
| | Organic | 303 | 76 | 0.6091 | −0.3400 | 0.0395 |
| cc-pVTZ | General | 118 | 30 | 0.3914 | −0.1875 | 0.0265 |
| | Organic | 308 | 77 | 0.3279 | −0.1640 | 0.0200 |
| cc-pVQZ | General | 118 | 30 | 0.2819 | −0.1234 | 0.0207 |
| | Organic | 308 | 77 | 0.2172 | −0.0947 | 0.0109 |

Table S3: Numbers of fit and test samples, fitted extrapolation parameters and MAEs on the test sets for qs$GW$ and different GTO basis sets.

| Basis Set | Molecules | $n_{\text{train}}$ | $n_{\text{test}}$ | $\alpha_0$ | $\alpha_1$ | MAE [eV] |
|---|---|---|---|---|---|---|
| cc-pVDZ | General | 124 | 32 | 0.4302 | −0.2532 | 0.0820 |
| | Organic | 211 | 53 | 1.0367 | −0.4359 | 0.0543 |
| cc-pVDZ | General | 124 | 32 | 0.4540 | −0.1827 | 0.0286 |
| | Organic | 211 | 53 | 0.4567 | −0.1809 | 0.0238 |
| cc-pVQZ | General | 124 | 32 | 0.1330 | −0.0538 | 0.0209 |
| | Organic | 211 | 53 | 0.1255 | −0.0506 | 0.0175 |

Table S4: Fitted extrapolation parameters for different STO basis sets for $G_0W_0$. For the General set, 128 train samples and 32 test samples were used. For the Organic set, 220 train samples and 56 test samples were used.

| Basis Set | Molecules | $\alpha_0$ | $\alpha_1$ | [eV] |
|---|---|---|---|---|
| TZ3P | General | 0.6670 | −0.2910 | 0.0516 |
| | Organic | 0.2999 | −0.1833 | 0.0334 |
| TZ2P | General | 0.7524 | −0.3350 | 0.0334 |
| | Organic | 1.0426 | −0.4068 | 0.0415 |
| TZP | General | 0.6345 | −0.3485 | 0.0509 |
| | Organic | 0.9184 | −0.4168 | 0.0418 |
| DZP | General | 0.2953 | −0.2322 | 0.0622 |
| | Organic | 1.2420 | −0.4340 | 0.0689 |

Table S5: Fitted extrapolation parameters for different STO basis sets for $\Sigma^{BSE}@L^{BSE}$. For the General set, 118 train samples and 30 test samples were used. For the Organic set, 308 train samples and 77 test samples were used.

| Basis Set | Molecules | $\alpha_0$ | $\alpha_1$ | MAE [eV] |
|---|---|---|---|---|
| TZ3P | General | 0.4710 | −0.2041 | 0.0432 |
| | Organic | 0.1336 | −0.0972 | 0.0176 |
| TZ2P | General | 0.4799 | −0.2220 | 0.0380 |
| | Organic | 0.6648 | −0.2576 | 0.0244 |
| TZP | General | 0.4116 | −0.2394 | 0.0429 |
| | Organic | 0.5977 | −0.2715 | 0.0307 |
| DZP | General | 0.1239 | −0.1217 | 0.0689 |
| | Organic | 0.7453 | −0.2162 | 0.0852 |

Table S6: Fitted extrapolation parameters for different STO basis sets for qs$GW$. For the General set, 124 train samples and 32 test samples were used. For the Organic set, 201 train samples and 55 test samples were used.

| Basis Set | Molecules | $\alpha_0$ | $\alpha_1$ | MAE [eV] |
|---|---|---|---|---|
| TZ3P | General | 0.8727 | −0.3137 | 0.0648 |
| | Organic | 0.6169 | −0.2355 | 0.0618 |
| TZ2P | General | 1.0519 | −-0.3866 | 0.0729 |
| | Organic | 1.9688 | −0.6209 | 0.0772 |
| TZP | General | 0.8496 | −0.3843 | 0.0881 |
| | Organic | 2.3400 | −0.7574 | 0.0830 |
| DZP | General | 0.4418 | −0.2535 | 0.0943 |
| | Organic | 1.5376 | −0.4929 | 0.1178 |

# BSIE Convergence

In the following we further validate our approach to use 5Z results as extrapolation targets for qs$GW$ calculations although the BSIE convergence is quite erratic, as mentioned in the main text. In Fig. S1 we show representative examples where the convergence is much faster than expected, much faster than expected and where the BSIE does not converge monotonously altogether. To confirm that this behavior is not merely a shortcoming of the method used by us we show results for qs$GW$ calculations with BHandHLYP, PBE0 and HF starting points. As can be seen in Fig. S1, all starting points agree on the same energies within only a few ten meV for the 5Z basis and not so for the QZ basis set.

We therefore tested if the erratic qs$GW$ BSIE convergence could be caused by our setting for the imaginary shift $\eta$ in Eq. 4 in the main text. Fig. S2, S3 and S4 show results exemplarily for HOCl, PN and $CH_4$ with different settings for $\eta$. The value of $\eta = 0.005$ Hartree is used throughout the main text. As can be seen, a higher value of $\eta = 0.01$ Hartree does have an influence on the overall BSIE convergence. However, while for HOCl (Fig. S2) the convergence behavior looks as

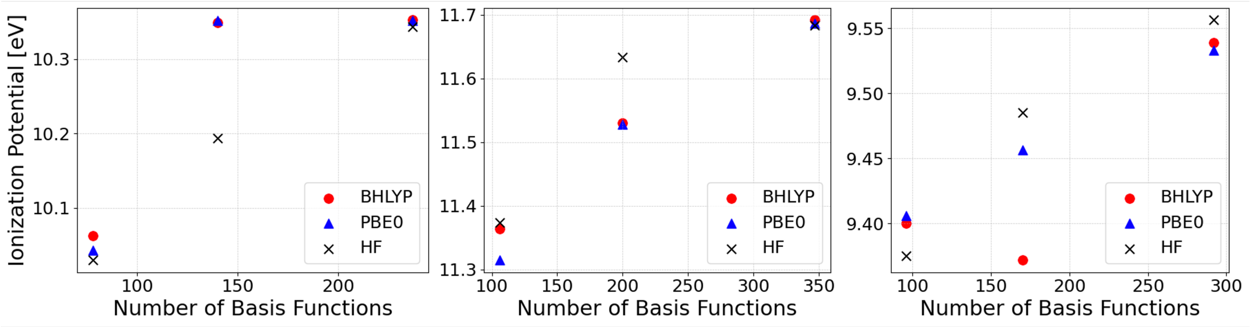


Figure S1: Ionization potential from qs*GW* calculations with BHandHLYP, PBE0 and HF starting points and TZ, QZ and 5Z basis sets for HOCl (left), $CH_3Cl$ (middle) and $P_2H_2$ (right) respectively.

generally expected with a higher value for $\eta$, both the other examples still do not correspond to the usually assumed convergence behavior as in both cases the convergence is much slower than expected. Furthermore, the standard deviations of the fitted extrapolation exponents over the qs*GW* remain high in comparison to those of $G_0W_0$ and $\Sigma^{BSE}@L^{BSE}$ even with the higher value for $\eta$. Similarly, the linear correlation between the natural logarithm of the kinetic energy and the BSIE does not seem to improve over the whole dataset. All in all, we therefore conclude that a higher value of $\eta$ has, as expected, a (somewhat positive) effect on the BSIE convergence behavior of qs*GW* for individual samples, however not to the extent needed for reliable CBS limit references and especially not for our whole fit set. While using an even higher value of $\eta$ could potentially solve the problem, it would lead to a sizable artificial shift in the QP energies. For this reason, we do not investigate this solution, and rely on 5Z calculations instead.

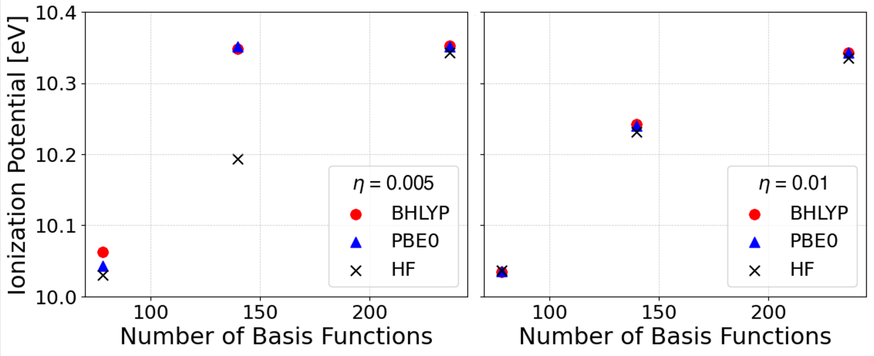


Figure S2: Ionization potential from qs*GW* calculations with BHandHLYP, PBE0 and HF starting points, TZ, QZ and 5Z basis sets and different imaginary shifts $\eta$ for HOCl.

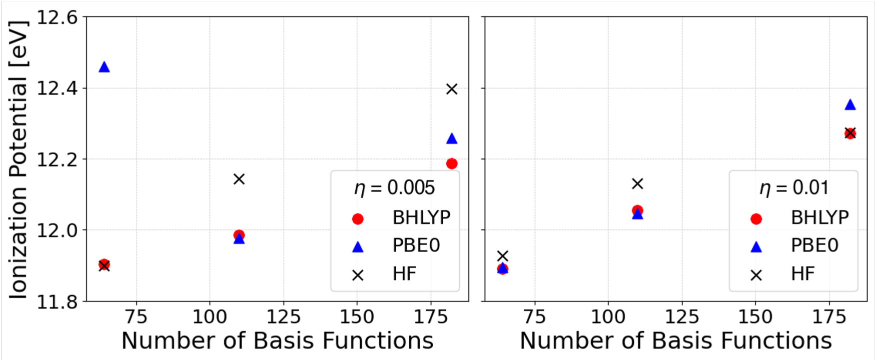


Figure S3: Ionization potential from qs*GW* calculations with BHandHLYP, PBE0 and HF starting points, TZ, QZ and 5Z basis sets and different imaginary shifts $\eta$ for PN.

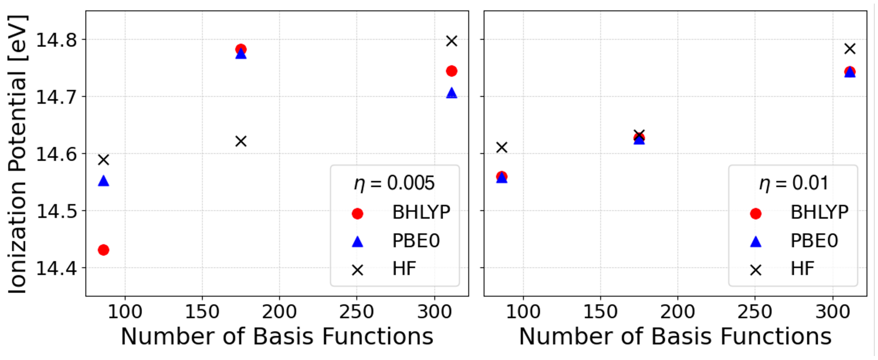


Figure S4: Ionization potential from qs*GW* calculations with BHandHLYP, PBE0 and HF starting points, TZ, QZ and 5Z basis sets and different imaginary shifts $\eta$ for $CH_4$.
